# Supplementary material for: Emerging two-dimensional conductivity at Mott-band insulator interface
Source: arXiv:2401.16813 source file (2024-01-30)
Supplement: Supplementary file 1 [file LTO-KTO-3interfaces-Suppl6.pdf]

# Supplemental Material: Emerging two-dimensional conductivity at Mott-band insulator interface

I. V. Maznichenko,[1,2,*] S. Ostanin,[1] D. Maryenko,[3] V. K. Dugaev,[4]
E. Ya. Sherman,[5,6] P. Buczek,[2] I. Mertig,[1] M. Kawasaki,[3,7] and A. Ernst[8,9]

[1]*Institute of Physics, Martin Luther University Halle-Wittenberg, D-06099 Halle, Germany*
[2]*Department of Engineering and Computer Sciences, Hamburg University of Applied Sciences, Berliner Tor 7, D-20099 Hamburg, Germany*
[3]*RIKEN Center for Emergent Matter Science(CEMS), Wako 351-0198, Japan*
[4]*Department of Physics and Medical Engineering, Rzeszów University of Technology, 35-959 Rzeszów, Poland*
[5]*Department of Physical Chemistry and the EHU Quantum Center, University of the Basque Country UPV/EHU, Bilbao 48080, Spain*
[6]*Ikerbasque, Basque Foundation for Science, Bilbao, Spain*
[7]*Department of Applied Physics and Quantum-Phase Electronics Center (QPEC), The University of Tokyo, Tokyo 113-8656, Japan*
[8]*Institute for Theoretical Physics, Johannes Kepler University, A-4040 Linz, Austria*
[9]*Max Planck Institute for Microstructure Physics, Weinberg 2, D-06120 Halle, Germany*

## I. METHOD

The electronic properties and structural optimization of $LaTiO_3$ (LTiO), $KTaO_3$ (KTO), and the LTiO/KTO interfaces were computed using the Vienna *Ab initio* Simulation Package (VASP)[1] within the Perdew-Burke-Ernzerhof generalized-gradient approximation[2] (GGA-PBE) to the exchange-correlation potential. The electron-ion interactions were described by projector-augmented wave (PAW) pseudopotentials. The valence configurations $4s^1 3p^6$, $2s^2 2p^4$ and $4s^2 3p^6 3d^4$ are used for K, O, and Ti, respectively. The Ta pseudopotential is in the $5p^6 6s^2 5d^3$ valence configuration which includes the semi-core $5p$ states. The pseudopotential for La is in the $5s^2 5p^6 5d^1 6s^2$ configuration, in which the $5s5p$ semi-core states are treated as valence states. The electron wave functions were represented by plane waves with a cutoff energy of 450 eV. Ionic relaxation of the LTiO/KTO superlattices were performed using the conjugate-gradient algorithm until the Hellmann-Feynman forces became less than $1.2 \times 10^{-2}$ eV/Å.

After relaxation of each LTiO/KTO superlattice the density of states (DOS) was computed using the tetrahedron method on the Γ-centered dense **k**-mesh. The DOS and band structure calculations, $E(\mathbf{k})$, were performed also in the presence of spin-orbit coupling using the non-collinear VASP option.[3]

## II. ELECTRONIC PROPERTIES OF BULK $LaTiO_3$ AND $KTaO_3$

For a band insulator KTO, the use of GGA-PBE yields reliably wide gap while the calculated equilibrium volume overestimates slightly its experimental value by 2.3%. Regarding the Mott insulator LTiO, it is well known that its calculation within the density functional theory (DFT) needs the DFT+$U$ parametrization[4], i.e. the appropriate correlation parameter $U$ applied to the $3d$ orbitals of Ti. The use of the VASP implementation[5] of DFT+$U$ and the effective parameter $U_{\text{eff}}$ = 2.3 eV gives for orthorhombic (*Pbnm*) lanthanum titanate (i) the band gap of 0.5 eV, (ii) the $G$-type antiferromagnetic structure and (iii) the Ti magnetic moment of 0.7 $\mu_B$. The similar results of the DFT+$U$ calculation of LTiO were reported previously.[6] Using the recently developed self-interaction cancellation leads to a band gap of 50 meV.[7]

The total and site-projected DOS of the cubic KTO are plotted in Figure 1 (left panel). The calculated band gap exceeds 2 eV and the Ta $5d$ states dominate in the low conduction band, whereas the upper valence band is formed by the O $p$ states.

The total and site-projected DOS of orthorombic $LaTiO_3$ are shown in Figure 1 (middle panel). Here, the 4-f.u.-cell (f.u. for formula unit) is needed to model the $D_{2h}$ structure with the O tilting and antiferromagnetically ordered Ti. The band gap of 0.48 eV separates the 0.57-eV occupied subband from the unoccupied conduction band edge $E_c$. The $3d$ Ti states form the both separated parts of the low conduction band. The $f$ states of La appear massively at higher energies starting from $E > E_c + 1.3$ eV. In this study, we do not correct the position of the La $f$-states and treat them with no $U$-parametrization. The latter may shift the unoccupied $f$-states of La to the higher energies. Accordingly to our calculation of $LaTiO_3$, each Ti has the magnetic moment of about $0.7\mu_B$. The Ti magnetic species are ordered antiferromagnetically to each other so that the $G$-type structure shows the lowest energy. The ferromagnetically ordered configuration of LTiO, which is unfavorable by 1.5 eV/f.u., shrinks the band gap to its marginal value of 50 meV.

The key structural factor of LTiO, which keeps its band gap and antiferromagnetism, is the optimally rotated $TiO_6$ octahedra. This peculiarity can be evaluated using the oxygen tilting. The O tilting angle $\theta$ is defined as the deviation from the direct line $B$–O–$B$ of cubic perovskite $ABO_3$. In orthorombic LTiO, $\theta$ = 26°. To explore the role of tilting in these systems, we inspected the electronic and magnetic properties of KTO and LTiO by changing its $\theta$ between zero and 32°.

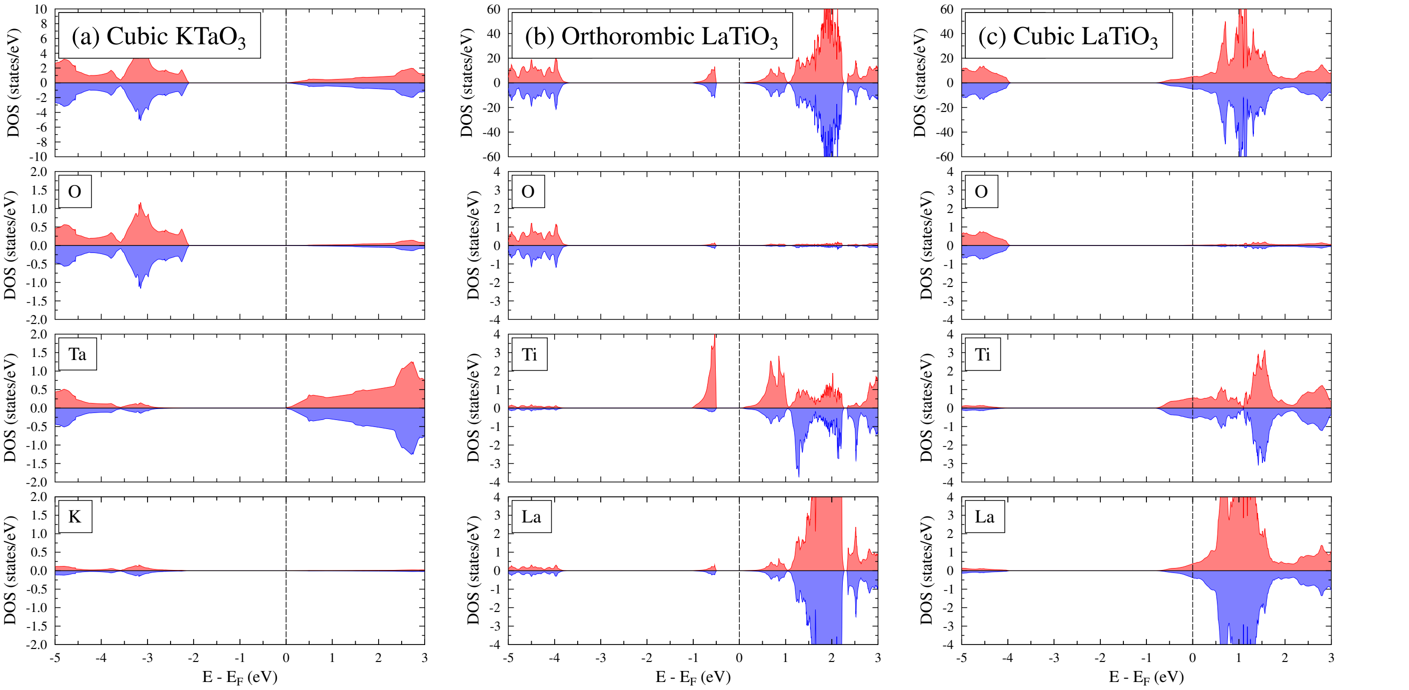


FIG. 1: Total and site-projected DOS of cubic $KTaO_3$ (left panel), orthorombic LTiO (middle panel), and cubic LTiO (right panel).

The spin-polarized DOS of untilted LTiO which is plotted in Figure 1 (right panel) illustrates that the untilted phase is metallic so that its $E_F$ is about 0.8 eV above the conduction band edge. The LTiO cell used here contains 4 f.u. For that reason and because of metallicity, the number of $E(\mathbf{k})$ which cross $E_F$ is rather large.

## III. (001), (110), AND (111) INTERFACES

Orthorhombic LTiO with lattice parameters $a = b = 5.595$ Å and $c = 7.912$ Å can be considered as a pseudocubic structure with the effective lattice constant $a_{pc} = \sqrt{a^2 + b^2}/2 \cong c/2 = 3.956$ Å, which differs by about 0.8% from that of cubic KTO, namely, $a = 3.989$ Å. The fact that perovskites grow in complete unit cells[8,9] determines the choice of the atomic order at the interfaces in the numerical calculations. To simulate LTiO/KTO (001) interfaces we constructed superlattices from the 8-f.u.-thick KTO (001) and 8-f.u.-thick LTiO (001) using the experimental lattice parameters of LTiO for the in-plane geometry, shown in Fig. 3. Position relaxation of the LTiO/KTO superlattices, being one of the key points in the 2DEG formation assured the Hellmann-Feynman forces $< 1.2\times10^{-2}$ eV/Å. To involve all degrees of freedom, which correspond to the oxygen tilting in LTiO and also to its $G$-type antiferromagnetism, we used the $\sqrt{2}a \times \sqrt{2}b$ in-plane geometry. Each (001) plane of the LTiO/KTO (001) supercell, therefore, contains two cations. The lattice mismatch between the materials in LTiO/KTO is relatively small. We inspected that the use of the LTiO lattice parameters affects the electronic properties of KTO only marginally. The 160-atom 8-f.u./8-f.u. supercell of LTiO/KTO (001) after relaxation is shown in Fig. 3. The $TiO_6$ and $TaO_6$ octahedra illustrate there how the bulk-like $TiO_6$ tilting seen in the deep LTiO layers weakens toward the interfaces, locks with the induced tilting of the $TaO_6$ octahedra and, then, almost disappears in the third u.c. of KTO. Interfacial $TiO_6$ and $TaO_6$ octahedra are shown in Fig. 4(a).

Each Ta atom at interface LTiO on $TaO_2$-terminated KTO (001) has 5 neighboring Ta atoms and only one Ti atom, whereas K/La ratio is 1:1, see Tab. I. The interfacial Ti has also only one Ta atom, but all cations type $A$ are La atoms.

For the LTiO/KTO (110) interface, we used mainly a 240-atom 8-f.u.-LTiO/4-f.u.-KTO supercell, which contains four f.u. of $ABO_3$ perovskite in each layer. The (111) interface was simulated using a 160-atom LTiO/KTO supercell, where each atomic layer contains the two f.u. of $ABO_3$. The 8-f.u.-thick KTO slab within the 320-atom supercell was inspected as well. The $TiO_6$ and $TaO_6$ octahedra at (110) and (111) interfaces are shown in Fig. 4(b) and Fig. 4(c), respectively. In contrast to (001) interface,

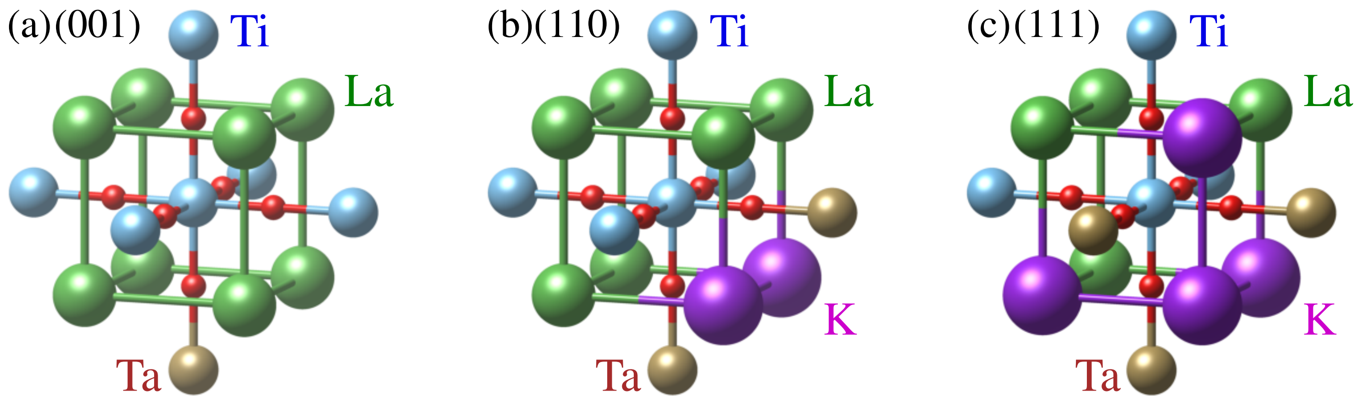


FIG. 2: Schematic presentation of the atomic structure close to (001), (110), and (111) interfaces with Ti(I+1) in the center: (a), (b), and (c), respectively. Next nearest neighbors of Ti at $TaO_2$-terminated KTO (001) are La atoms, whereas K atoms are presented for (110) and (111). For more details see Table I.

TABLE I: Number of neighbors and average concentrations for interfacial Ta(I) and Ti(I+1).

| | Ta(I) | | | | | | Ti(I+1) | | | | | |
|---|---|---|---|---|---|---|---|---|---|---|---|---|
| Interface | Ta | Ti | Ti(%) | K | La | La(%) | Ta | Ti | Ta(%) | K | La | K(%) |
| (001) | 5 | 1 | 16.7 | 4 | 4 | 50 | 1 | 5 | 16.7 | 0 | 8 | 0 |
| (110) | 4 | 2 | 33.3 | 6 | 2 | 33.3 | 2 | 4 | 33.3 | 2 | 6 | 33.3 |
| (111) | 3 | 3 | 50 | 4 | 4 | 50 | 3 | 3 | 50 | 1 | 7 | 12.5 |

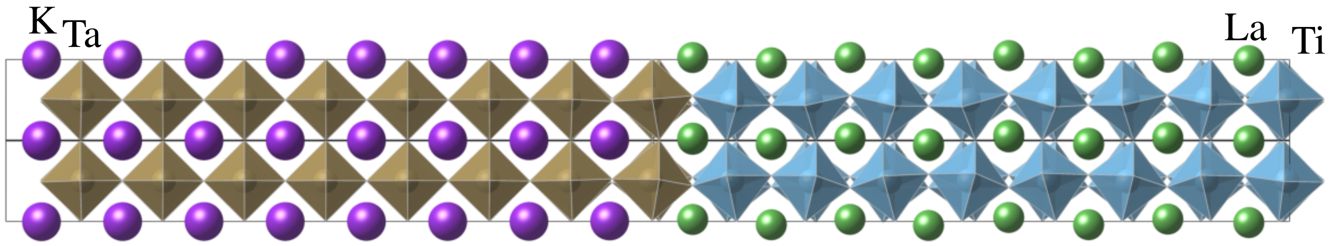


FIG. 3: Relaxed crystal structure of the 8-f.u.-$LaTiO_3$/8-f.u.-$KTaO_3$ (001) superlattice. The $TaO_6$ and $TiO_6$ octahedra are shown in red and blue, respectively.

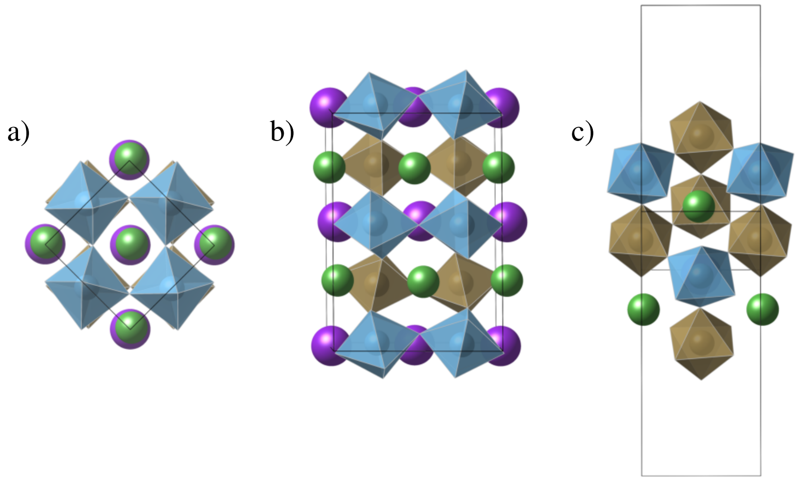


FIG. 4: Interfacial LTiO/KTO configurations of the (001), (110), and (111) interfaces, which are plotted in the (a), (b) and (c) panels, respectively. La is shown in green, K in magenta, O in red. The $TaO_6$ and $TiO_6$ octahedra are shown in brown and blue, respectively.

the concentration of foreign atoms at interface is much higher: 33% and 50% for (110) and (111), respectively, see Tab. I.

* Electronic address: igor.maznichenko@physik.uni-halle.de

[1] G. Kresse and J. Furthmüller, Phys. Rev. B **54**, 11169 (1996).
[2] J. P. Perdew, K. Burke, and M. Ernzerhof, Phys. Rev. Lett. **77**, 3865 (1996).
[3] D. Hobbs, G. Kresse, and J. Hafner, Phys. Rev. B **62**, 11556 (2000).
[4] V. I. Anisimov, J. Zaanen, and O. K. Andersen, Phys. Rev. B **44**, 943 (1991).
[5] A. Rohrbach, J. Hafner, and G. Kresse, Journal of Physics: Condensed Matter **15**, 979 (2003).
[6] H.-S. Ahn, D. D. Cuong, J. Lee, and S. Han, Journal of the Korean Physical Society **49**, 1536 (2006).
[7] J. Varignon, M. Bibes, and A. Zunger, Phys. Rev. B **100**, 035119 (2019).
[8] H. L. Meyerheim, F. Klimenta, A. Ernst, K. Mohseni, S. Ostanin, M. Fechner, S. Parihar, I. V. Maznichenko, I. Mertig, and J. Kirschner, Phys. Rev. Lett. **106**, 087203 (2011).
[9] R. Guo, L. Tao, M. Li, Z. Liu, W. Lin, G. Zhou, X. Chen, L. Liu, X. Yan, H. Tian, et al., Science Advances **7** (2021).
